# Supplementary material for: From Small-World Networks to Comparison-Based Search
Source: arXiv:1107.3059 source file (2014-02-10)
Supplement: Supplementary file 1 [file appendix.tex]

%\techrepfix{}{
\section{Proof of Theorem~\protect\lowercase{\ref{hardnessthm}}}\label{proof:hardness}
\input{hardness_short}
%\input{hardness}
%}

%\input{nonmetric}
